# Supplementary material for: Dipolar spin-waves and tunable band gap at the Dirac points in the 2D magnet ErBr3
Source: arXiv:2206.10168 source file (2022-06-21)
Supplement: Supplementary file 1 [file ErBr3_-_C.Wessler_-_Supplementary_Information.pdf]

# Dipolar spin-waves and tunable band gap at the Dirac points in the 2D magnet $\text{ErBr}_3$

Christian Wessler<sup>1,2\*</sup>, Bertrand Roessli<sup>1</sup>, Karl W. Krämer<sup>3</sup>, Uwe Stuhr<sup>1</sup>,

Andrew Wildes<sup>4</sup>, Hans B. Braun<sup>3</sup> and Michel Kenzelmann<sup>1,2</sup>

<sup>1</sup>Laboratory for Neutron Scattering and Imaging,

Paul Scherrer Institut, Villigen, Switzerland

<sup>2</sup>Department of Physics, Universität Basel, Basel, Switzerland

<sup>3</sup>Department of Chemistry, Biochemistry, and  
Pharmacy, University of Bern, Bern, Switzerland

<sup>4</sup>Institut Laue-Langevin, Grenoble, France

\*To whom correspondence should be addressed; E-mail: christian.wessler@psi.ch

## Supplementary information

### Supplementary Note 1: Dipolar interactions

The dipolar sum in Fourier space was performed using Ewald's method [1, 2] which guarantees a fast convergence of lattice sums. We tested our calculations against those of Johnston [3] for 2D and 3D dipolar lattices and found an excellent agreement with his results. Results of the calculations for the  $\text{ErBr}_3$  structure, with six ions in the chemical cell, are presented in Supplementary Figure 1 and Supplementary Figure 2. The dispersion of the eigenvalues of the dipolar tensor is presented in Supplementary Figure 1 and the dependence of the largest eigenvalue as a function of the lattice parameter  $c$  is shown in Supplementary Figure 2. Mean-field calculations of the dispersion of the eigenvalues of the Fourier transform of the dipolar tensor for the R-3 chemical structure of  $\text{ErBr}_3$  with 6 ions in the cell show that the magnetic structure retains continuous degeneracy. The dispersion of the highest eigenvalues is flat along the  $c$ -direction, as shown below, which confirms that  $\text{ErBr}_3$  (with lattice parameter  $c = 18.89 \text{ \AA}$ ) is well inside the two-dimensional (2D) limit (see Supplementary Figure 3), in agreement with the observation of a rod of magnetic scattering

at  $\kappa = (1/3, 1/3, L)$  in neutron diffraction (see Supplementary Figure 4).

### Supplementary Note 2: Crystalline electric-field splitting

When an  $f$ -ion is embedded in a crystal, the surrounding charges influence the free-ion electronic energy levels and wave functions. If the electrostatic potential is sufficiently weak so that the splitting of the  $(2J + 1)$  electronic levels of the  $^{2S+1}L_J$  ground-state can be treated as a perturbation, the crystalline electric-field Hamiltonian can be written as a sum over angular momentum operators

$$H_{CEF} = \sum_{n=0}^6 \sum_{m=0}^n B_n^m O_n^m.$$

The  $B_n^m$  are the parameters which have to be determined from experiment, whereas the  $O_n^m$  are the Stevens operators [4]. Although the general CEF operator might have up to 27 independent parameters (because  $B_n^m$  with  $m \neq 0$  can be complex), the electrostatic potential reflects the point symmetry of the rare-earth site. Hence, depending on symmetry, some of the CEF parameters are equal to zero [5]. For the trigonal point symmetry  $C_3$  of the  $\text{Er}^{3+}$  site in  $\text{ErBr}_3$ , the data was analyzed on the basis of the CEF operator

$$\begin{aligned} H_{CEF} = & B_2^0 O_2^0 + \\ & B_4^0 O_4^0 + B_4^{+3} O_4^{+3} + B_4^{-3} O_4^{-3} + \\ & B_6^0 O_6^0 + B_6^{+3} O_6^{+3} + B_6^{-3} O_6^{-3} + B_6^{+6} O_6^{+6} + B_6^{-6} O_6^{-6} \end{aligned}$$

which splits the non-perturbed ground-state  $J = 15/2$  of  $\text{Er}^{3+}$  into 8 Kramers doublets.

The CEF-splitting can be measured by INS [6] and the result of such an inelastic spectrum taken at  $T = 1.5$  K is shown in Supplementary Figure 5. Three magnetic excitations are observed at  $E \sim 1.5$  meV, 3.0 meV and 6.2 meV which correspond to transitions from the lowest CEF level to the excited CEF levels of the  $^4\text{I}_{15/2}$  ground state. The line shows the result of a least-square fit to the data that resulted in the CEF-parameters of Supplementary Table 1. We also used measurements of the static susceptibility to determine the CEF-parameters as shown in the inset of Supplementary Figure 5. We could reproduce the

temperature dependence of the static magnetic susceptibility with  $\chi_a = \chi_b \sim 3 \chi_c$  at  $T = 1.5$  K using the parameters shown in Supplementary Table 2 which give CEF-levels at 0 meV, 1.48 meV, 3.82 meV, 6.69 meV, 13.71 meV, 16.59 meV, 19.75 meV and 20.77 meV.

### Supplementary Note 3: Spin waves

In Supplementary Figure 6 a and b, we show a selection of INS scans along  $(0, q, 0)$  and at  $\Gamma$ , M and K points. The calculation of the inelastic neutron cross-section of the spin-waves was performed in the magnetic Brillouin zone, see Supplementary Figure 6c. The single-ion susceptibility was calculated with [7]

$$\chi_0^{\alpha, \beta}(E) = \sum_{i, j} \frac{\langle i | S_\alpha | j \rangle \langle j | S_\beta | i \rangle}{(E_j - E_i - E)^2 + \Gamma^2} \Gamma (n_i - n_j),$$

where  $i, j$  are the eigenstates and  $E_i, E_j$  the eigenvalues of the mean-field Hamiltonian;  $S_\alpha, S_\beta$  are the components of the spin operators in Cartesian coordinates.  $n_i, n_j$  are the Boltzmann occupation factors and  $\Gamma$  the linewidth. We note that the calculation of  $S(\kappa, E)$  is parameter free as the value for the magnetic moment of  $\text{Er}^{3+}$   $\mu = 4.7\mu_B$  used for the calculation was determined in Ref. [8] by neutron diffraction and the easy-plane anisotropy caused by the CEF is taken into account by anisotropic  $g$ -factors [9]. For  $\text{ErBr}_3$ , we obtained  $g_x = g_y = 9.4$  and  $g_z = 0.1$  which reflects the large easy-plane anisotropy at  $T = 80$  mK.

The dispersion of the spin-waves is obtained by solving the equation  $\det[\bar{1} - \bar{\chi}_0(E) \bar{\bar{D}}(\mathbf{q})] = 0$ . We find that the stiffness of the acoustic branch depends on the angle  $\Psi$  as shown in Supplementary Figure 7. In agreement with the results of Prakash and Henley for the dipolar honeycomb antiferromagnet, the acoustic magnon branch is soft at  $\Psi = 30^\circ, 90^\circ, 150^\circ, 210^\circ, 270^\circ$  and  $330^\circ$  (see Supplementary Figure 7c) The spin configurations corresponding to these values of  $\Psi$  are selected by thermal fluctuations [10].

### Supplementary Note 4: Berry phase and Berry curvature

The Berry phase  $\gamma$  was calculated on a small closed circle around the  $K$ -point using

$$\gamma = -\Im \log[\langle u(\mathbf{k}_0)|u(\mathbf{k}_1)\rangle\langle u(\mathbf{k}_1)|u(\mathbf{k}_2)\rangle\ldots\langle u(\mathbf{k}_{N-1})|u(\mathbf{k}_N)\rangle]$$

where  $|u(\mathbf{k}_i)\rangle$  is the magnon eigenvector at point  $\mathbf{k}_i$  and  $|u(\mathbf{k}_N)\rangle = |u(\mathbf{k}_0)\rangle$  as detailed in Ref. [11]. The eigenvectors were determined by solving the matrix equation [12]

$$[\bar{1} - \bar{\chi}_0(E)\bar{D}(\mathbf{k}_i)]|u(\mathbf{k}_i)\rangle = 0$$

with a *svd* algorithm. The Berry curvature  $\Omega(\mathbf{k})$  was computed with the method proposed by Fukui *et al.* [13]. The Chern number is the integral of  $\Omega(\mathbf{k})$  divided by  $2\pi i$ . Supplementary Figure 8 presents the evolution of the Berry curvature as a function of  $\Psi$ .

- 
- [1] Cohen, M.H. & Keffer, F. Dipolar sums in the primitive cubic lattices. *Phys. Rev.* **99**, 1128 (1955).
  - [2] Bowden, G.J. & Clark, R.G. Fourier transforms of dipole-dipole interactions using Ewald's method. *J. Phys. C: Solid State Phys.* **14**, L827 (1981).
  - [3] Johnston, D.C. Magnetic dipole interactions in crystals. *Phys. Rev. B* **93**, 014421 (2016).
  - [4] Stevens, K.W.H. Matrix elements and operator equivalents connected with the magnetic properties of rare earth ions. *Proc. Phys. Soc. A* **65**, 209 (1952).
  - [5] Bauer, E. & Rotter, M. *Magnetism of complex metallic alloys: crystalline electric field effects*, in: Book Series on Complex Metallic Alloys Vol. 2, ed. E. Belin-Ferr, World Scientific (2009).
  - [6] Fulde, P. & Loewenhaupt, M. Magnetic excitations in crystal-field split 4f systems. *Adv. Physics* **34**, 589 (1985).
  - [7] Jensen, J. & Macintosh, A.R. *Rare earth magnetism*, Clarendon Press, Oxford (1991).
  - [8] Krämer, K.W. *et al.* Noncollinear two- and three-dimensional magnetic ordering in the honeycomb lattices of  $\text{ErX}_3$  (X=CL,Br,I). *Phys. Rev. B* **60**, R3724 (1999).
  - [9] Rastelli, E. *Statistical mechanics of magnetic excitations*, Series on Advances in Statistical Mechanics – Vol. 18, World Scientific. (2013).

- [10] Prakash, S. & Henley, C.L. Ordering due to disorder in dipolar magnets on two-dimensional lattices. *Phys. Rev. B* **10**, 6574 (1990).
- [11] Vanderbilt, D. *Berry phases in electronic structure theory*, Cambridge University Press (2018).
- [12] Thalmeier, P. Low-energy Nd spin waves in noncollinear Nd<sub>2</sub>CuO<sub>4</sub>. *Physica C* **266**, 89 (1996).
- [13] Fukui, T., Hatsugai, Y. & Suzuki, H. Chern numbers in discretized Brillouin zone: Efficient method of computing (spin) Hall conductances. *J. Phys. Soc. Jpn.* **74**, 1674 (2005).

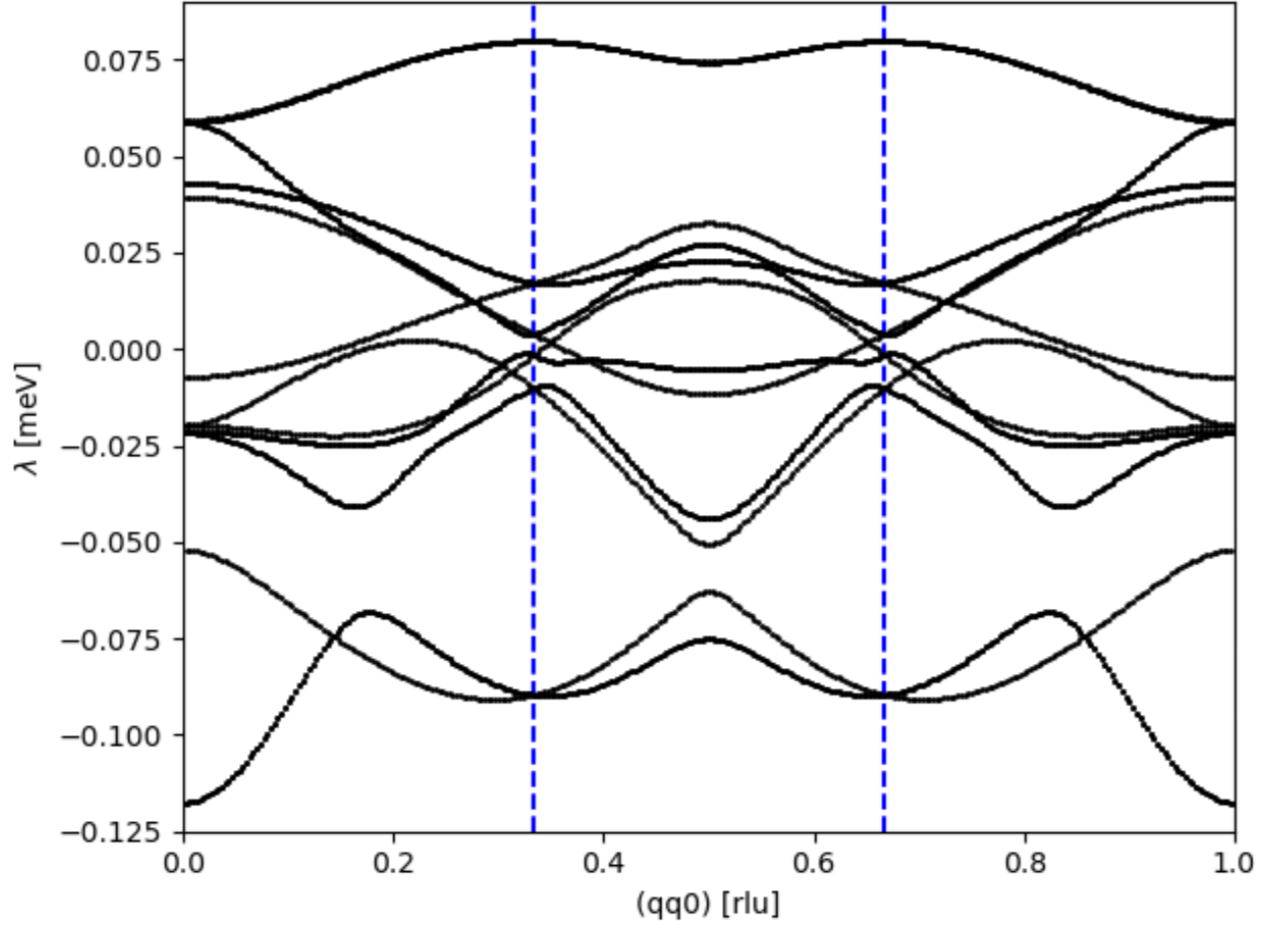

Supplementary Figure 1: Dispersion of the eigenvalues of the Fourier transform of the dipolar tensor which shows a maximum at  $\mathbf{k}_0 = (1/3, 1/3, 0)$  and at  $(2/3, 2/3, 0)$  that is equivalent to  $(-1/3, -1/3, 0)$ .

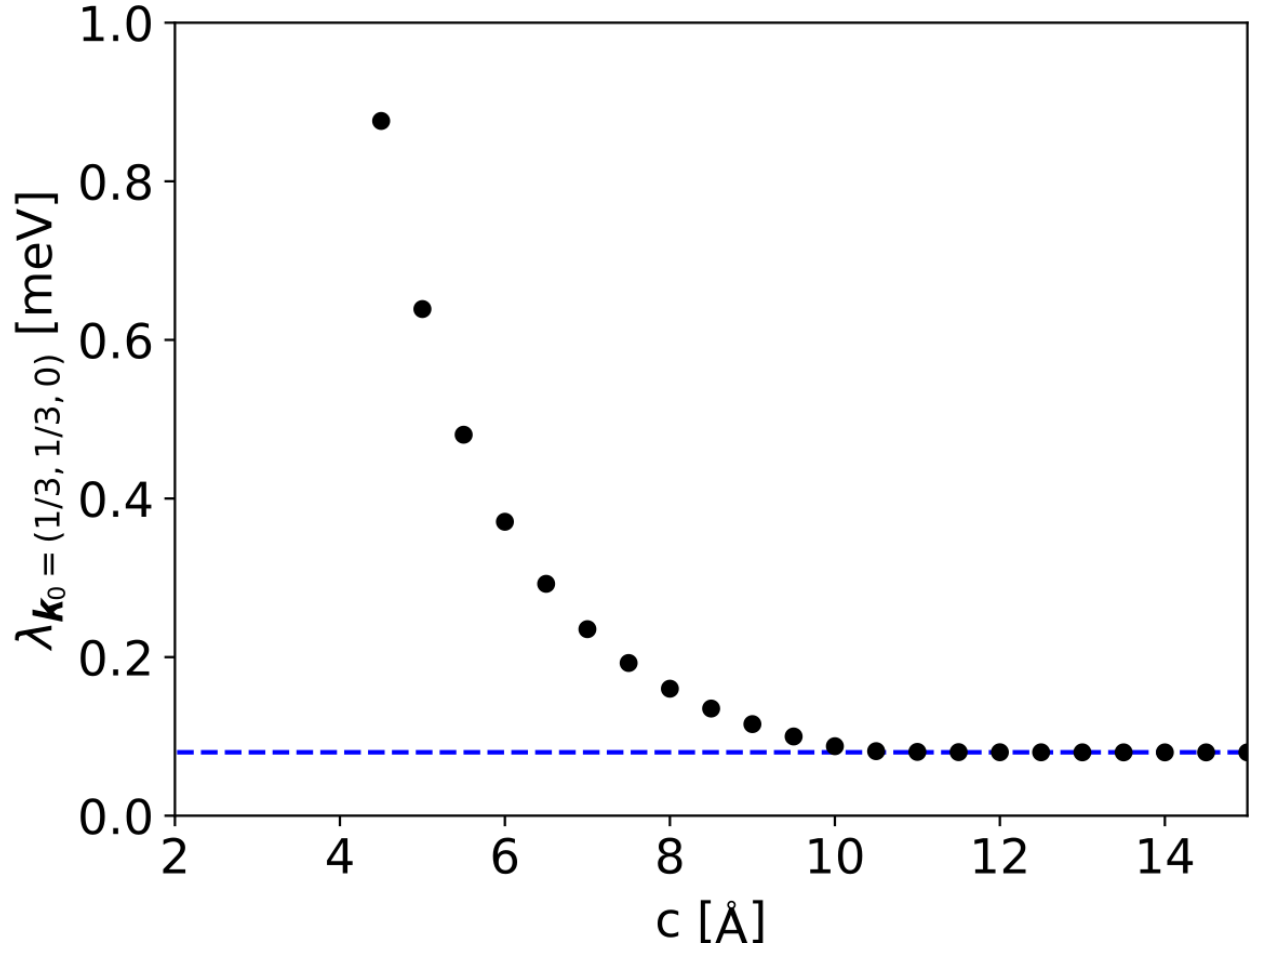

Supplementary Figure 2: Dependence of the largest eigenvalue on the lattice parameter  $c$ .  $\text{ErBr}_3$  with  $c = 18.89 \text{ \AA}$  is well in the 2D limit [3].

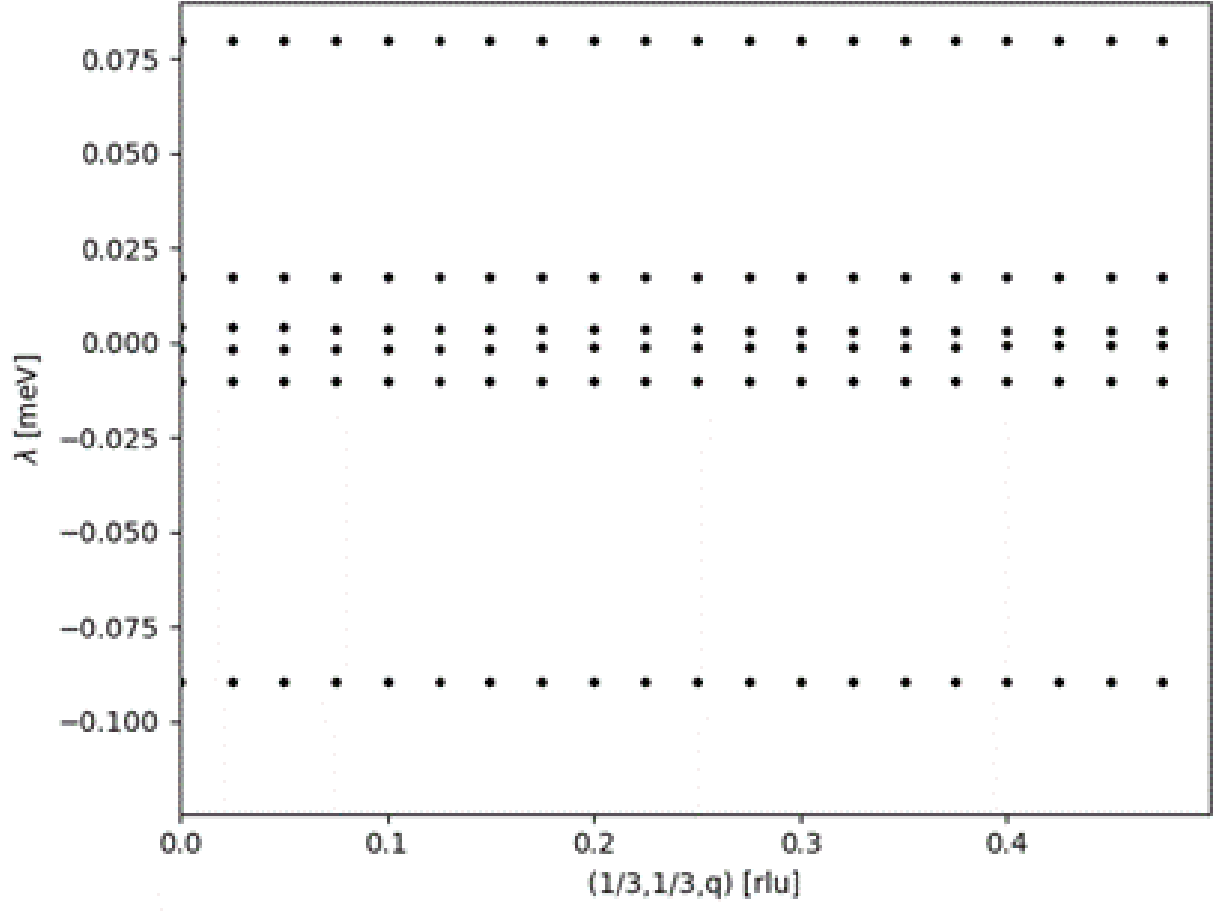

Supplementary Figure 3: Dispersion of the eigenvalues of the Fourier transform of the dipolar tensor for  $\text{ErBr}_3$  with the R-3 structure along the  $c$ -direction. Note that the eigenvalues are degenerate.

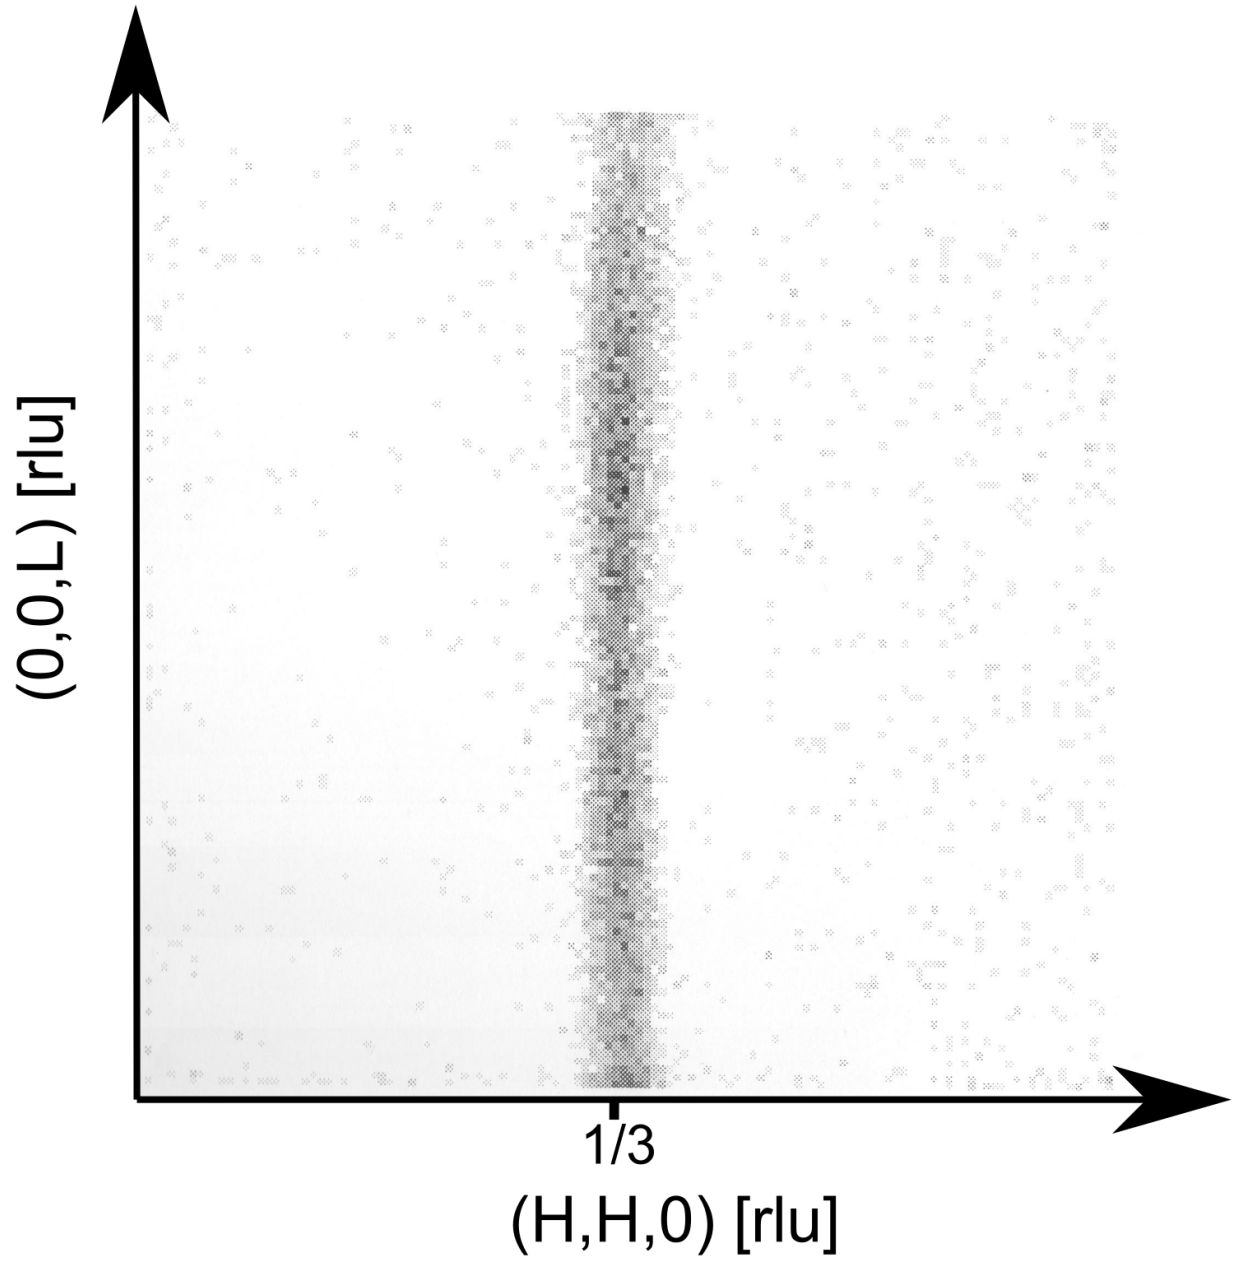

Supplementary Figure 4: Magnetic scattering in the  $(H, H, L)$ -plane of  $\text{ErBr}_3$ .

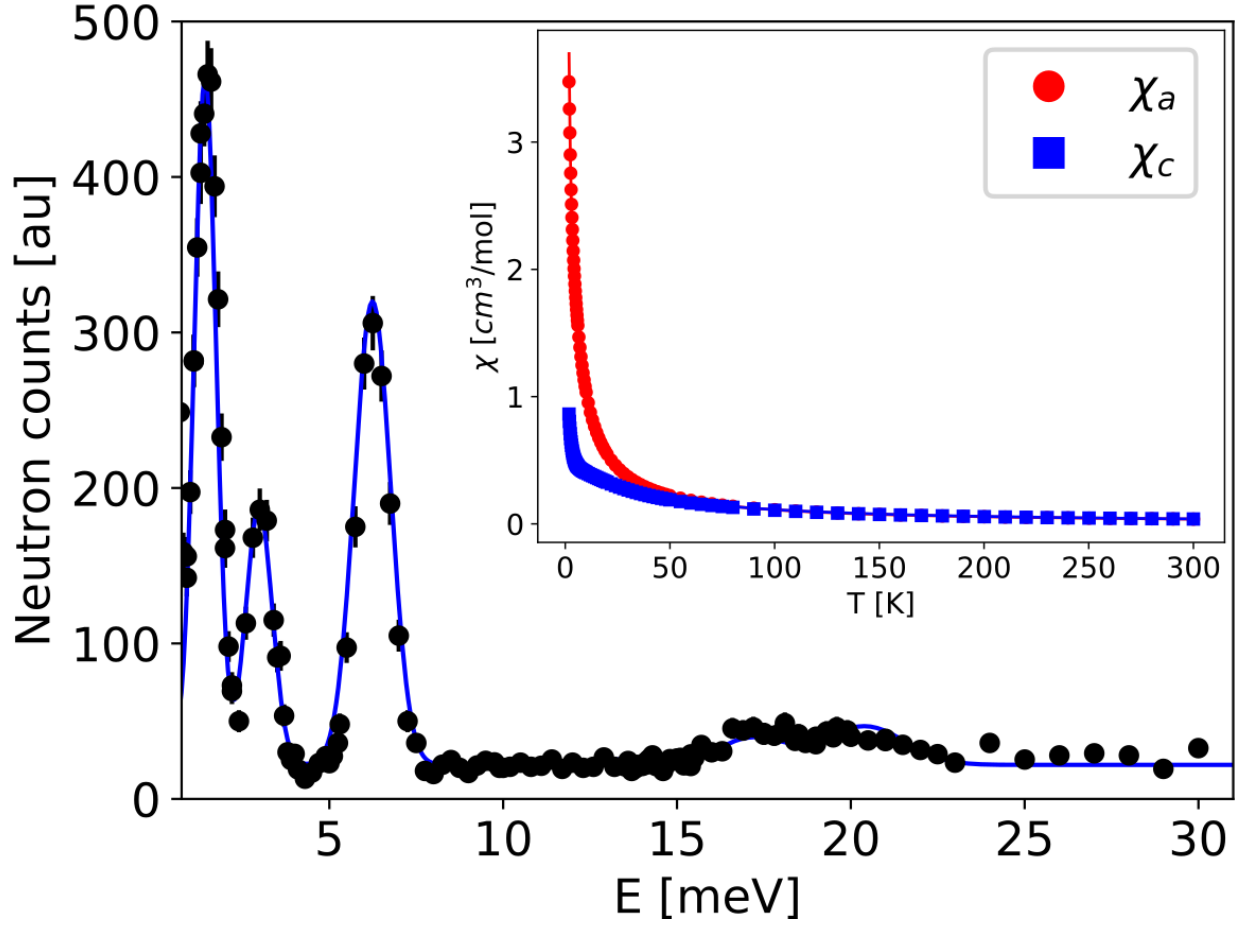

Supplementary Figure 5: Crystalline electric-field splitting in  $\text{ErBr}_3$  measured by INS at  $T = 1.5$  K. The temperature dependence of the static susceptibility is shown in the inset. The lines result from the calculations explained in the text. Error bars are standard deviations.

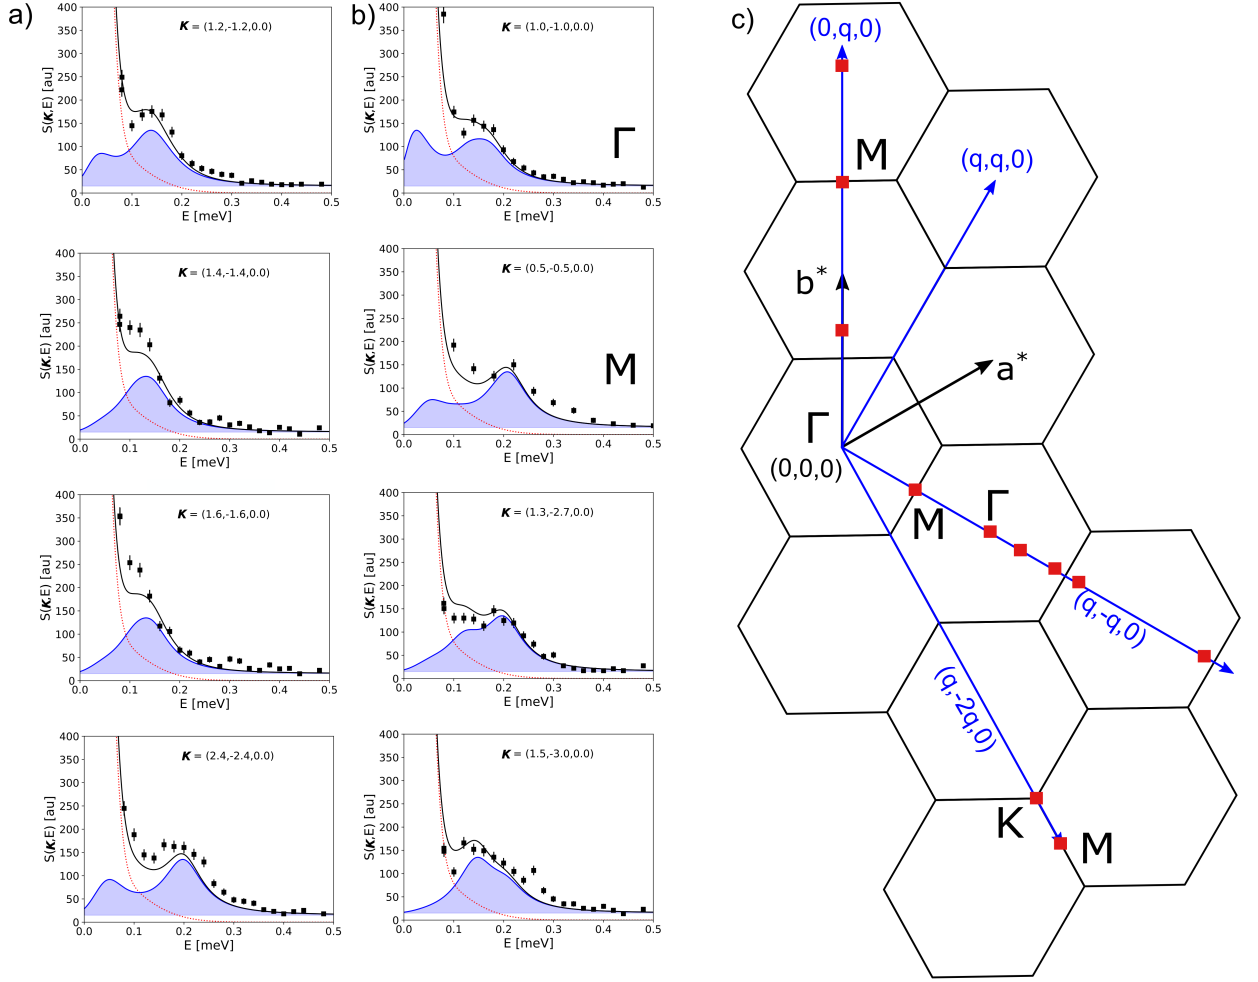

Supplementary Figure 6: a) Representative energy scans along the  $(q,-q,0)$  direction together with simulations of the inelastic neutron scattering cross-section shown as blue lines. The red line is a fit of the incoherent scattering measured at  $\mathbf{q} = (2/3, -4/3, 0)$  at  $T = 6$  K. The sum of both contributions is shown by the black line. b) As in a) for  $\Gamma$ , M and K. c) Extended magnetic Brillouin zone showing the different scan directions of the measurements and simulations. The red squares indicate the positions in reciprocal space of the scans shown in Fig. 2 and

Supplementary Figure 6. Error bars are standard deviations.

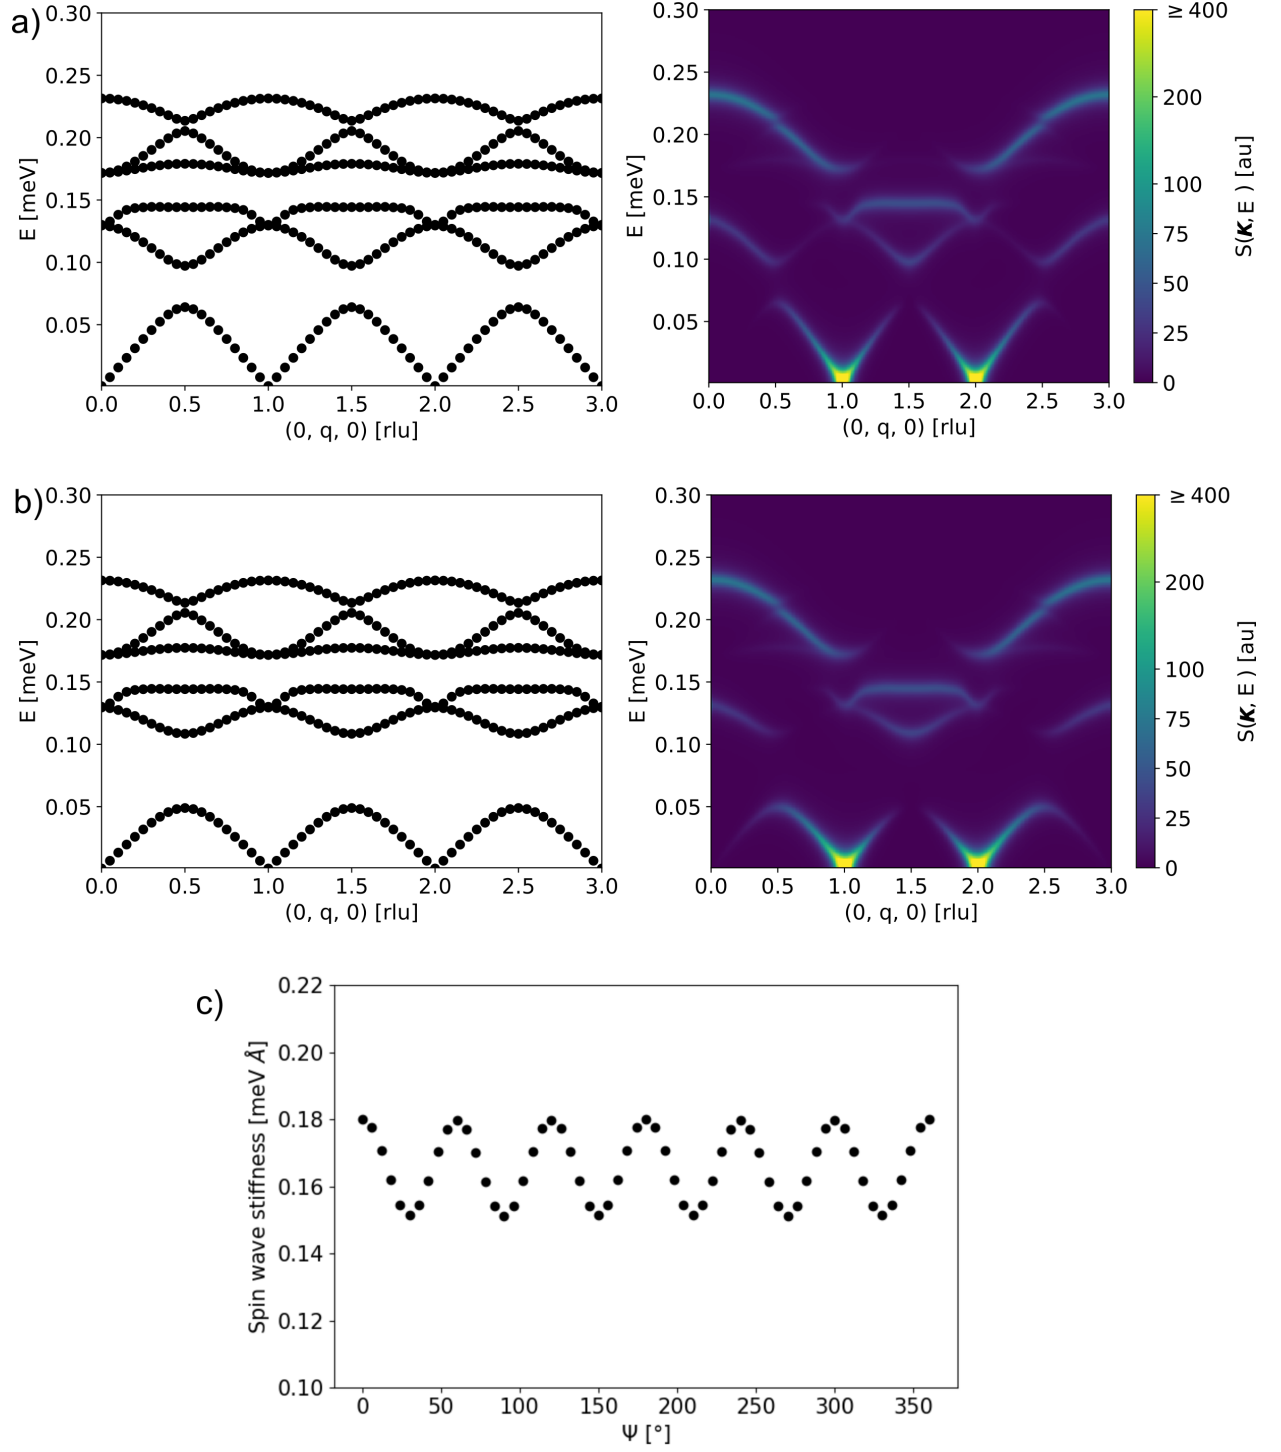

Supplementary Figure 7: Dispersion of the spin wave excitations calculated with MF-RPA along  $\mathbf{\kappa} = (0, q, 0)$  for the easy-plane honeycomb lattice with dipolar interactions for a)  $\Psi = 0$  and b)  $\Psi = 30^\circ$ . The color plots give the intensity of the inelastic neutron cross-section  $S(\mathbf{\kappa}, E)$ . c) Dependence of the spin-wave stiffness of the acoustic branch as a function of  $\Psi$ .

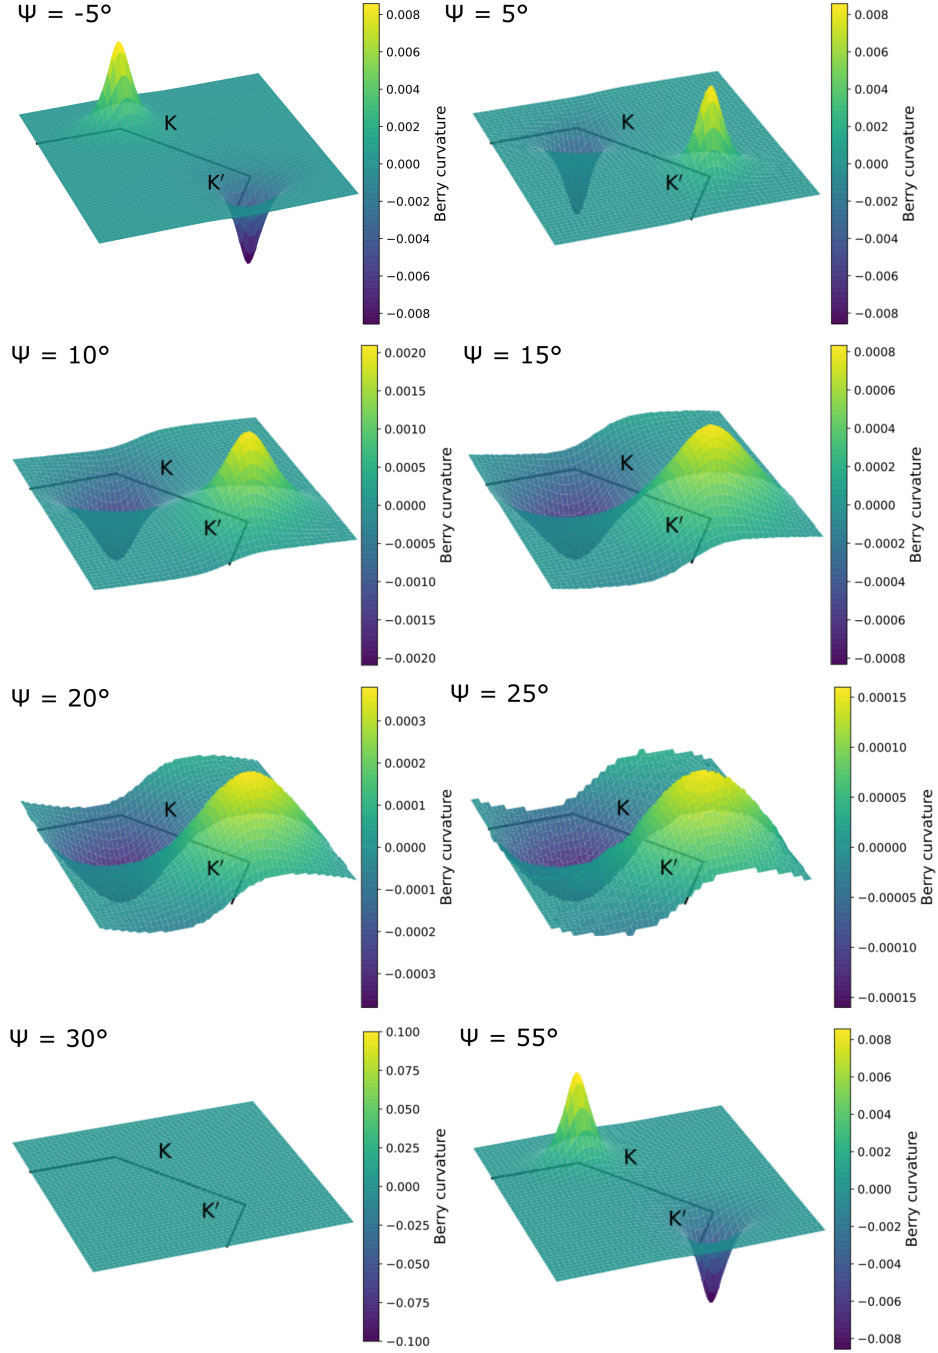

Supplementary Figure 8: Calculation of the Berry curvature for different  $\Psi$ . The Berry curvature has a period of  $\Psi = 60^\circ$ . As the value of  $\Psi = 30^\circ$  (where the gap is maximal) is approached, the Berry curvature progressively broadens and weakens with increasing  $\Psi$ .

| $B_2^0$ | $B_4^0$ | $B_4^{+3}$ | $B_4^{-3}$ | $B_6^0$ | $B_6^{+3}$ | $B_6^{-3}$ | $B_6^{+6}$ | $B_6^{-6}$ |
|---------|---------|------------|------------|---------|------------|------------|------------|------------|
| -7.35   | 6.1     | 0.01       | 9.2        | 0.45    | 6.17       | 14.8       | 32.8       | 17.4       |

Supplementary Table 1: CEF parameters  $B_n^m$  (in meV) for ErBr<sub>3</sub> obtained from the INS data.

| $B_2^0$ | $B_4^0$ | $B_4^{+3}$ | $B_4^{-3}$ | $B_6^0$ | $B_6^{+3}$ | $B_6^{-3}$ | $B_6^{+6}$ | $B_6^{-6}$ |
|---------|---------|------------|------------|---------|------------|------------|------------|------------|
| -7.80   | 6.69    | 6.78       | 12.29      | 0.42    | 7.59       | 22.22      | 8.453      | 32.63      |

Supplementary Table 2: CEF parameters  $B_n^m$  (in meV) for ErBr<sub>3</sub> obtained from the static susceptibility.
